# Supplementary material for: Evidence that PUBO outperforms QUBO when solving continuous optimization problems with the QAOA
Source: arXiv:2305.03390 source file (2023-05-05)
Supplement: Supplementary file 1 [file appendix.tex]

% \subsection{Discretization}\label{AppxDiscrete}
% All computational numerics require discretization. For us, this means binary discretization due to the architecture of Gate-Based Quantum Computing. For our functions, we introduced the following discretization on the input domain:
% \\
% We want to map from our input domain, to a bit string where each bit represents a power of 2, using the result of \eqref{binProof1}, where n represents the number of bitstrings (eg. n = 3 $\mapsto{}$ '000'). In order to reach decimal-place resolution, we will define Bit-resolution as the number of negative powers we take 2 to. For example, Bit-resolution 1 $\mapsto{} 2^{-1}$ and Bit-resolution 2 $\mapsto{} (2^{-1}+2^{-2})$. The result of \eqref{binProof2} justifies this usage.
% \begin{align*}
%     \sum_{i=0}^{n}{2^i} & =2^{n+1}-1 \numberthis\label{binProof1}\\
%     \lim_{k\rightarrow-\infty}\sum_{i=k}^{n}{2^i} & =2^{n+1} \numberthis\label{binProof2}
% \end{align*}
% Now, we need to map from an input domain [a,b], to n in \eqref{binProof1} (Although we define finding n below, we would still need further bits to define resolution and zero. These will be addressed later in \eqref{bitstringDom}).
% \\\\For Input Domain $[a,b]\in\mathbb{R}$, $a<b$:
% \begin{align*}
% n: \mathbb{R}\times\mathbb{R} &\rightarrow \mathbb{Z}\\ \numberthis \label{domBitLen}
% (a,b) &\mapsto{} {\lfloor{\ln_{2}{|max\{a,b\}|}}\rfloor} 
% \end{align*}
% And to keep track of negative domains, we define c as the negative domain flag:
% \begin{align*}
% c&\coloneqq\mathbb{I}_{\{a<0\}} \numberthis \label{negDomFlag}\\
% \\\mathbb{I}_{\{a<0\}}&\coloneqq
%  \begin{cases}
%       1 & \text{if $a<0$}\\
%       0 & \text{otherwise} 
%     \end{cases}
% \end{align*}
% We finally have all the ingredients to develop our bitstring:\\
% Using the formalism
% \begin{align*}
%     \text{Alphabet}&  &\Sigma&=\{0,1\}\\
%     \text{Kleene star}& &\Sigma^*&=\bigcup^\infty_{i=0}\Sigma^i\\\\
%     \text{Norm}& &\text{$|$ . $|$  :  }\Sigma^* &\rightarrow\mathbb{N}
% \end{align*}\\
% For a bitstring of length k:\\
% \begin{align*}
%     \{0,1\}^k \coloneqq \{x\in\{0,1\}^* : |x|=k\}
% \end{align*}\\
% For example $\{0,1\}^2$ = $\{00,01,10,11\}$.\\\\
% As such, we define our mapping from input domain [a,b], for Bit-resolution r, n \eqref{domBitLen}, c \eqref{negDomFlag}, to a bitstring $\mathbb{S}$ as:\\\\
% Let $\alpha\coloneqq n+c+r+1$
% \begin{align*}
% \mathbb{S} &\in \{0,1\}^{\alpha}\numberthis \label{bitstringDom}\\
% \mathbb{S} &\coloneqq s_{0}s_{\alpha-1}s_{\alpha-2}...s_{1}\numberthis \label{bitstringDef}
% \end{align*}
% Where the bit order is flipped, and 
% \begin{align*}
%     s_{0}=
%     \begin{cases}
%         \{0,1\} & \text{if c = 1 \eqref{negDomFlag}}\\
%         \varnothing & \text{if c = 0 \eqref{negDomFlag}}
%     \end{cases}
% \end{align*}
% For example, 2 $\in$ [0,3] $\mapsto{}$ '01' where the bit order is flipped, and 2 $\in$ [-3,3] $\mapsto{}$ '001', to be read as '0-01', where the zeroth bit is reserved for the negative flag. That is, -2 $\in$ [-3,3] $\mapsto{}$ '101'.\\\\
% Example of a two variable domain: 
% \\Let (x,y) $\in$ [-3,3]$\times$[-3,3]. Then x=3, y=2 $\mapsto{}$ '011001', to be read as '0-11', '0-01'; and x=3, y=2 $\in$ [-3,3]$\times$[0,3] $\mapsto{}$ '01101', to be read as '0-11', '01'.
